# Supplementary material for: Measurement of the Generalized Polarizabilities of the Proton at Intermediate $Q^2$
Source: arXiv:2008.08958 source file (2021-02-11)
Supplement: Supplementary file 1 [file README.pdf]

H.Fonvieille, LPC-Clermont-Fd, France  
August 2020

## SUPPLEMENTAL MATERIAL

to the Article:

“Measurement of the Generalized Polarizabilities of the Proton at Intermediate  $Q^2$ ”

### • Directories:

The three subdirectories Q2-0.10-GeV2, Q2-0.20-GeV2, and Q2-0.45-GeV2 contain the cross-section data of the experiment, for the photon electroproduction process  $ep \rightarrow ep\gamma$ . There is one subdirectory per value of  $Q^2$ .

In each subdirectory, files in ascii format contain cross-section data per bin in  $q'_{c.m.}$ . Each file is labelled by the value of  $q'_{c.m.}$  at the center of the bin:

|                                           |                                                   |
|-------------------------------------------|---------------------------------------------------|
| $q'_{c.m.} \in (25,50) \text{ MeV}/c :$   | $q'_{c.m.} \text{ central} = 37.5 \text{ MeV}/c$  |
| $q'_{c.m.} \in (50,75) \text{ MeV}/c :$   | $q'_{c.m.} \text{ central} = 62.5 \text{ MeV}/c$  |
| $q'_{c.m.} \in (75,100) \text{ MeV}/c :$  | $q'_{c.m.} \text{ central} = 87.5 \text{ MeV}/c$  |
| $q'_{c.m.} \in (100,125) \text{ MeV}/c :$ | $q'_{c.m.} \text{ central} = 112.5 \text{ MeV}/c$ |
| $q'_{c.m.} \in (125,150) \text{ MeV}/c :$ | $q'_{c.m.} \text{ central} = 137.5 \text{ MeV}/c$ |
| $q'_{c.m.} \in (150,175) \text{ MeV}/c :$ | $q'_{c.m.} \text{ central} = 162.5 \text{ MeV}/c$ |

For instance, the file q2-0.10-cross-sections-binqpr-37.5.txt contains data at  $q'_{c.m.} = 37.5 \text{ MeV}/c$  (and  $Q^2 = 0.10 \text{ GeV}^2$ ).

At  $Q^2 = 0.10 \text{ GeV}^2$ , five bins in  $q'_{c.m.}$  are filled, i.e., from 37.5 to 137.5 MeV/c.

At  $Q^2 = 0.10$  and  $0.20 \text{ GeV}^2$ , six bins in  $q'_{c.m.}$  are filled, i.e., from 37.5 to 162.5 MeV/c.

### • File content:

Each file has 1440 lines, corresponding to (36 bins in  $\phi_{c.m.} \times 40$  bins in  $\cos\theta_{c.m.}$ ). Each line contains 12 numbers, corresponding to:

---

|                                               |                                                                                                                   |
|-----------------------------------------------|-------------------------------------------------------------------------------------------------------------------|
| column 1 :                                    | value of $q_{c.m.}$ in MeV/ $c$                                                                                   |
| column 2 :                                    | value of $q'_{c.m.}$ in MeV/ $c$                                                                                  |
| column 3 :                                    | value of virtual photon polarization $\epsilon$                                                                   |
| column 4 :                                    | value of $\cos \theta_{c.m.}$                                                                                     |
| column 5 :                                    | value of $\phi_{c.m.}$ in degrees                                                                                 |
| column 6 :                                    | value of the measured cross section $d\sigma_{\text{exp}}$ , in pb/(MeV.sr <sup>2</sup> )                         |
| column 7 :                                    | value of the statistical error $\Delta d\sigma_{\text{exp}}(stat.)$ <sup>(*)</sup> , in pb/(MeV.sr <sup>2</sup> ) |
| The next five columns contain auxiliary data: |                                                                                                                   |
| column 8 :                                    | coefficient $V_{LL}$ of the LEX in Eq.(3)                                                                         |
| column 9 :                                    | coefficient $V_{LT}$ of the LEX in Eq.(3)                                                                         |
| column 10 :                                   | (BH+Born) cross section <sup>(**)</sup> in pb/(MeV.sr <sup>2</sup> )                                              |
| column 11 :                                   | example of a GP term $(\Phi q'_{c.m.})\Psi_0$ <sup>(***)</sup>                                                    |
| column 12 :                                   | phase-space factor $(\Phi q'_{c.m.})$ in Eq.(3)                                                                   |

---

(\*) at one standard deviation.

(\*\*) : calculated with the proton form-factor parametrization of Ref.[24] (J.Friedrich and T.Walcher, EPJA 17 (2003) 607).

(\*\*\*) : calculated with arbitrary values of the structure functions  $P_{LL} - P_{TT}/\epsilon$  and  $P_{LT}$  (not necessarily the final ones).

The kinematics of the  $ep \rightarrow ep\gamma$  reaction is entirely determined by the values in the first five columns, i.e., by  $(q_{c.m.}, q'_{c.m.}, \epsilon, \cos \theta_{c.m.}$  and  $\phi_{c.m.})$ . The symbol  $d\sigma_{\text{exp}}$  stands for  $d^5\sigma_{\text{exp}}/(dE'_e d\Omega'_e d\cos\theta_{c.m.} d\phi_{c.m.})$  (cf. the article).

#### • Empty bins:

In the first 720 lines of each file, corresponding to values of  $\phi_{c.m.}$  in the range  $(-180^\circ, 0^\circ)$ , **there is no measured cross section, i.e., the cross section is equal to -1 and the error is equal to 0**. Only the lines 721 to 1440, corresponding to  $\phi_{c.m.} \in (0^\circ, +180^\circ)$  may contain a valid measurement; this is because the cross section has been symmetrized in  $\phi_{c.m.}$ . A valid cross-section point is therefore identified by a number in the 6th column different from -1 and a number in the 7th column different from 0.

Cross sections presented in the files are obtained after collecting the cross-section data measured for each kinematical setting separately, and “merging” them. This operation of “merging” is necessary since some of the 3D-bins receive events from several settings. In such a case, we take the weighed average of the several cross section values.

#### • About the $q'_{c.m.}$ -bins:

The LEX fit uses only three  $q'_{c.m.}$ -bins below the pion production threshold:  $q'_{c.m.} = 62.5, 87.5$  and  $112.5$  MeV/ $c$ .

The DR fit may use the additional bins  $q'_{c.m.} = 137.5$  and  $162.5$  MeV/ $c$  which are above the pion production threshold.

The lowest  $q'_{c.m.}$ -bin (37.5 MeV/ $c$ ) is used for normalization tests.

#### • Absolute normalization and total error:

An uncertainty of  $\pm 1.5$  % relative is attached to each measured cross-section, to be understood as a global normalization uncertainty, acting on the whole data set.

The statistical error on each cross-section point is given by  $\pm\Delta d\sigma_{\text{exp}}(\text{stat.})$  in the data files. The systematic error is given by:  $\Delta d\sigma_{\text{exp}}(\text{syst.}) = (\pm 0.015) \cdot d\sigma_{\text{exp}}$ . If one wants the total error on the cross section, one has to make the quadratic sum of these two contributions.
